# Supplementary material for: Arena Learning: Build Data Flywheel for LLMs Post-training via Simulated Chatbot Arena
Source: arXiv:2407.10627 source file (2024-07-15)
Supplement: Supplementary file 1 [file Appendix.tex]

% \newpage
